# Supplementary material for: Construction of a Validated Virtual Embodiment Questionnaire
Source: arXiv:1911.10176 ancillary file (2019-11-25)
Supplement: Supplementary file 1 [file audioinstructions-english4.pdf]

**Audio Instructions.**

*Each instruction followed by a pause to give the participant time to investigate and perceive.*

*The instructions were initially presented in german and were preliminary translated.*

**Study 1: Immersion**

|                                                                                                                                        |
|----------------------------------------------------------------------------------------------------------------------------------------|
| Stand relaxed, let your arms hang relaxed.                                                                                             |
| You will now receive some audio instructions to follow.                                                                                |
| Please conscientiously perform only the movements specified in the audio instructions and try not to get distracted during this phase. |
| We will now begin with the tasks.                                                                                                      |
| Hold your right arm straight forward with your palm facing down.                                                                       |
| Look at your right hand.                                                                                                               |
| Look at the same hand in the reflection.                                                                                               |
| Put your arm comfortably back down and look at your reflection.                                                                        |
| Hold your left arm straight forward with your palm facing down.                                                                        |
| Look at your left hand.                                                                                                                |
| Look at the same hand in the reflection.                                                                                               |
| Put your arm comfortably back down and look at your reflection.                                                                        |
| Put your right hand in front of your chest, the palm is facing downwards.                                                              |
| Look at your right hand.                                                                                                               |
| Look at the same hand in the reflection.                                                                                               |
| Put your arm comfortably back down next to your hip and look at your reflection.                                                       |
| Put your left hand in front of your chest, the palm is facing downwards.                                                               |
| Look at your left hand.                                                                                                                |
| Look at the same hand in the reflection.                                                                                               |
| Put your arm comfortably back down next to your hip and look at your reflection.                                                       |
| Stand relaxed.                                                                                                                         |
| Look at your feet and take two small steps backwards.                                                                                  |
| Stand relaxed and look forwards at your reflection.                                                                                    |
| Look at your feet and take two small steps forwards.                                                                                   |

## **Study 2: User-performed Personalization**

|                                                                                                                                        |
|----------------------------------------------------------------------------------------------------------------------------------------|
| Stand relaxed, let your arms hang relaxed.                                                                                             |
| You will now receive some audio instructions to follow.                                                                                |
| Please conscientiously perform only the movements specified in the audio instructions and try not to get distracted during this phase. |
| We will now begin with the tasks.                                                                                                      |
| Hold your right arm straight forward with your palm facing down.                                                                       |
| Look at your right hand.                                                                                                               |
| Look at the same hand in the reflection.                                                                                               |
| Put your arm comfortably back down and look at your reflection.                                                                        |
| Hold your left arm straight forward with your palm facing down.                                                                        |
| Look at your left hand.                                                                                                                |
| Look at the same hand in the reflection.                                                                                               |
| Put your arm comfortably back down and look at your reflection.                                                                        |
| Put your right hand with some distance in front of your chest, the palm is facing downwards.                                           |
| Look at your right hand.                                                                                                               |
| Look at the same hand in the reflection.                                                                                               |
| Put your arm comfortably back down next to your hip and look at your reflection.                                                       |
| Put your left hand with some distance in front of your chest, the palm is facing downwards.                                            |
| Look at your left hand.                                                                                                                |
| Look at the same hand in the reflection.                                                                                               |
| Put your arm comfortably back down next to your hip and look at your reflection.                                                       |
| Stand relaxed.                                                                                                                         |
| Take two small steps forward.                                                                                                          |
| Look at your reflection.                                                                                                               |
| Look at the face of your reflection.                                                                                                   |
| Look at the eye area of your reflection.                                                                                               |
| Look at the mouth area of your reflection.                                                                                             |

|                                                                                                                             |
|-----------------------------------------------------------------------------------------------------------------------------|
| Take two small steps back.                                                                                                  |
| Turn 90 degrees to the left and look over your right shoulder at the reflection.                                            |
| Turn back 90 degrees to the right. Turn another 90 degrees to the right and look at the left shoulder of your mirror image. |
| Turn back 90 degrees to the left.                                                                                           |
| Stand relaxed.                                                                                                              |
| Please stand still for a moment. The experimenter will now assist you in removing the VR glasses.                           |

### **Study 3: Behavioral Realism**

|                                                                                                                                        |
|----------------------------------------------------------------------------------------------------------------------------------------|
| Stand relaxed on the shown marker. Let your arms hang relaxed.                                                                         |
| You will now receive some audio instructions to follow.                                                                                |
| Please conscientiously perform only the movements specified in the audio instructions and try not to get distracted during this phase. |
| We will now begin with the tasks.                                                                                                      |
| Hold your right arm straight forward with your palm facing down.                                                                       |
| Look at your right hand.                                                                                                               |
| Look at the same hand in the reflection.                                                                                               |
| Put your arm comfortably back down and look at your reflection.                                                                        |
| Hold your left arm straight forward with your palm facing down.                                                                        |
| Look at your left hand.                                                                                                                |
| Look at the same hand in the reflection.                                                                                               |
| Put your arm comfortably back down and look at your reflection.                                                                        |
| Put your right hand with some distance in front of your chest, the palm is facing downwards.                                           |
| Look at your right hand.                                                                                                               |
| Look at the same hand in the reflection.                                                                                               |
| Put your arm comfortably back down next to your hip and look at your reflection.                                                       |
| Put your left hand with some distance in front of your chest, the palm is facing downwards.                                            |
| Look at your left hand.                                                                                                                |
| Look at the same hand in the reflection.                                                                                               |

|                                                                                                                                                                                                                        |
|------------------------------------------------------------------------------------------------------------------------------------------------------------------------------------------------------------------------|
| Put your arm comfortably back down next to your hip and look at your reflection.                                                                                                                                       |
| Stand relaxed.                                                                                                                                                                                                         |
| Walk forward to the next marker shown.                                                                                                                                                                                 |
| Look at your reflection.                                                                                                                                                                                               |
| Fixate with the eyes the left eye of your reflection.                                                                                                                                                                  |
| Fixate with the eyes the right ear of your reflection.                                                                                                                                                                 |
| Fixate with the eyes the nose of your reflection.                                                                                                                                                                      |
| Fixate with the eyes the right eye of your reflection.                                                                                                                                                                 |
| Stand relaxed.                                                                                                                                                                                                         |
| Now open your mouth, about halfway, and look at your reflection.                                                                                                                                                       |
| Close your mouth again.                                                                                                                                                                                                |
| Try to imitate a cheerful look by smiling at your reflection and look at your reflection.                                                                                                                              |
| Return to a neutral facial expression and look at your reflection.                                                                                                                                                     |
| Please repeat the following sentence slowly, looking at your reflection: "Blaukraut bleibt Blaukraut und Brautkleid bleibt Brautkleid."<br><br>Red cabbage remains red cabbage and bridal gown remains bridal gown. :D |
| Stand relaxed.                                                                                                                                                                                                         |
| Please stand still for a moment. The experimenter will now assist you in removing the VR glasses.                                                                                                                      |

#### **Study 4-Latency**

|                                                                               |
|-------------------------------------------------------------------------------|
| Stand relaxed, let your arms hang relaxed.                                    |
| You will now receive some audio instructions. Please follow the instructions. |
| Try not to get distracted during this phase.                                  |
| We will now begin with the tasks.                                             |
| Hold your right arm straight forward with your palm facing down.              |
| Look at your right hand.                                                      |
| Look at the same hand in the reflection.                                      |
| Put your arm comfortably back down and look at your reflection.               |
| Hold your left arm straight forward with your palm facing down.               |

|                                                                                                                                                               |
|---------------------------------------------------------------------------------------------------------------------------------------------------------------|
| Look at your left hand.                                                                                                                                       |
| Look at the same hand in the reflection.                                                                                                                      |
| Put your arm comfortably back down and look at your reflection.                                                                                               |
| Put your right hand in front of your chest, the palm is facing downwards.                                                                                     |
| Look at your right hand.                                                                                                                                      |
| Look at the same hand in the reflection.                                                                                                                      |
| Put your arm comfortably back down next to your hip and look at your reflection.                                                                              |
| Put your left hand in front of your chest, the palm is facing downwards.                                                                                      |
| Look at your left hand.                                                                                                                                       |
| Look at the same hand in the reflection.                                                                                                                      |
| Put your arm comfortably back down next to your hip and look at your reflection.                                                                              |
| Stand relaxed.                                                                                                                                                |
| Now stretch your left arm forward at moderate speed and put it back down next to your hip. Repeat this movement 10 times and look at your arm.                |
| Stand relaxed.                                                                                                                                                |
| Now stretch your right arm forward at moderate speed and put it back down next to your hip. Repeat this movement 10 times and look at your reflection.        |
| Stand relaxed.                                                                                                                                                |
| Point with your right hand 10 times at moderate speed first diagonally to the left shoulder of your reflection and then to the right foot of your reflection. |
| Put your right arm comfortably back down next to your hip and look at your reflection.                                                                        |
| Point with your left hand 10 times at moderate speed first diagonally to the right shoulder of your reflection and then to the left foot of your reflection.  |
| Put your arm comfortably back down next to your hip.                                                                                                          |
| Stand relaxed.                                                                                                                                                |
| This run is now complete.                                                                                                                                     |
| The experimenter will now assist you in removing the head-mounted display.                                                                                    |
